# Supplementary material for: Cold-Start Recommendation towards the Era of Large Language Models (LLMs): A Comprehensive Survey and Roadmap
Source: arXiv:2501.01945 source file (2025-01-16)
Supplement: Supplementary file 1 [file 9_appendix.tex]

\appendix
\section{Paper Overview}
In this part, we will provide a detailed overview of existing papers, categorized by our taxonomy. More resources on existing cold-start recommendation works can be found in our Github repository: \textcolor{blue}{\url{https://github.com/YuanchenBei/Awesome-Cold-Start-Recommendation}}.

%\resizebox{\linewidth}{!}{

\subsection{Content Features}
% Table generated by Excel2LaTeX from sheet 'Sheet1'
% Table generated by Excel2LaTeX from sheet 'Sheet1'
\begin{table}[htbp]
  \centering
  \caption{Overview of representative content feature-based cold-start recommendation papers.}
  \resizebox{\linewidth}{!}{
    \begin{tabular}{c|ll|c|c}
    \toprule
    Content Feature & \multicolumn{2}{c|}{Paper} & Volume & Cold-Start Task \\
    \midrule
    \multirow{37}[16]{*}{\rotatebox{90}{Data-Incomplete Learning}} & \multicolumn{4}{c}{Robust Co-Training} \\
\cmidrule{2-5}          & \multicolumn{2}{l|}{Temporally and Distributionally Robust Optimization for Cold-Start Recommendation} & AAAI24 & ItemCS \\
          & \multicolumn{2}{l|}{Collaborative Filtering in Latent Space: A Bayesian Approach for Cold-Start Music Recommendation} & PAKDD24 & UserCS \\
          & \multicolumn{2}{l|}{GoRec: A Generative Cold-Start Recommendation FrameworkGoRec: A Generative Cold-Start Recommendation Framework} & MM23  & ItemCS \\
          & \multicolumn{2}{l|}{Transform Cold-Start Users into Warm via Fused Behaviors in Large-Scale Recommendation} & SIGIR22 & UserCS* \\
          & \multicolumn{2}{l|}{Improving Item Cold-start Recommendation via Model-agnostic Conditional Variational Autoencoder} & SIGIR22 & ItemCS \\
          & \multicolumn{2}{l|}{Alleviating Cold-start Problem in CTR Prediction with A Variational Embedding Learning Framework} & WWW22 & CS \\
          & \multicolumn{2}{l|}{Zero Shot on the Cold-Start Problem: Model-Agnostic Interest Learning for Recommender Systems} & CIKM21 & UserCS \\
          & \multicolumn{2}{l|}{Recommendation for New Users and New Items via Randomized Training and Mixture-of-Experts Transformation} & SIGIR20 & CS \\
          & \multicolumn{2}{l|}{How to Learn Item Representation for Cold-Start Multimedia Recommendation?} & MM20  & ItemCS \\
          & \multicolumn{2}{l|}{From Zero-Shot Learning to Cold-Start Recommendation} & AAAI19 & UserCS \\
          & \multicolumn{2}{l|}{DropoutNet: Addressing Cold Start in Recommender Systems} & NIPS17 & CS \\
\cmidrule{2-5}          & \multicolumn{4}{c}{Knowledge Alignment} \\
\cmidrule{2-5}          & \multicolumn{2}{l|}{Preference Aware Dual Contrastive Learning for Item Cold-Start Recommendation} & AAAI24 & ItemCS \\
          & \multicolumn{2}{l|}{CMCLRec: Cross-modal Contrastive Learning for User Cold-start Sequential Recommendation} & SIGIR24 & UserCS \\
          & \multicolumn{2}{l|}{Aligning Distillation For Cold-start Item Recommendation} & SIGIR23 & ItemCS \\
          & \multicolumn{2}{l|}{Contrastive Collaborative Filtering for Cold-Start Item Recommendation} & WWW23 & ItemCS \\
          & \multicolumn{2}{l|}{Self-supervised Contrastive Enhancement with Symmetric Few-shot Learning Towers for Cold-start News Recommendation} & CIKM23 & CS* \\
          & \multicolumn{2}{l|}{Contrastive Learning for Cold-Start Recommendation} & MM21  & ItemCS \\
          & \multicolumn{2}{l|}{Generative Adversarial Framework for Cold-Start Item Recommendation} & SIGIR22 & ItemCS \\
          & \multicolumn{2}{l|}{Generative Adversarial Zero-Shot Learning for Cold-Start News Recommendation} & CIKM22 & CS \\
          & \multicolumn{2}{l|}{Revisiting Cold-Start Problem in CTR Prediction: Augmenting Embedding via GAN} & CIKM22 & UserCS \\
          & \multicolumn{2}{l|}{Cold \& Warm Net: Addressing Cold-Start Users in Recommender Systems} & DASFAA23 & UserCS \\
\cmidrule{2-5}          & \multicolumn{4}{c}{Cold Exploration} \\
\cmidrule{2-5}          & \multicolumn{2}{l|}{ColdNAS: Search to Modulate for User Cold-Start Recommendation} & WWW23 & UserCS* \\
          & \multicolumn{2}{l|}{Meta Policy Learning for Cold-Start Conversational Recommendation} & WSDM23 & UserCS \\
          & \multicolumn{2}{l|}{User Cold-start Problem in Multi-armed Bandits: When the First Recommendations Guide the User’s Experience} & TORS23 & UserCS* \\
          & \multicolumn{2}{l|}{Reinforcement Learning to Optimize Lifetime Value in Cold-Start Recommendation} & CIKM21 & ItemCS* \\
\cmidrule{2-5}          & \multicolumn{4}{c}{Feature Similarity Measurement} \\
\cmidrule{2-5}          & \multicolumn{2}{l|}{Automatic Fusion Network for Cold-start CVR Prediction with Explicit Multi-Level Representation} & ICDE23 & Long-tail \\
          & \multicolumn{2}{l|}{Cross-Modal Content Inference and Feature Enrichment for Cold-Start Recommendation} & IJCNN23 & Long-tail \\
          & \multicolumn{2}{l|}{SMINet: State-Aware Multi-Aspect Interests Representation Network for Cold-Start Users Recommendation} & AAAI22 & Long-tail \\
          & \multicolumn{2}{l|}{Content-aware Neural Hashing for Cold-start Recommendation} & SIGIR20 & ItemCS \\
          & \multicolumn{2}{l|}{Multi-Feature Discrete Collaborative Filtering for Fast Cold-start Recommendation} & AAAI20 & UserCS \\
          & \multicolumn{2}{l|}{Solving Cold-Start Problem in Large-scale Recommendation Engines: A Deep Learning Approach} & BigData16 & ItemCS \\
          & \multicolumn{2}{l|}{Collaborative Topic Modeling for Recommending Scientific Articles} & KDD11 & ItemCS \\
          & \multicolumn{2}{l|}{Deep pairwise hashing for cold-start recommendation} & TKDE20 &  \\
    \midrule
    \multirow{24}[20]{*}{\rotatebox{90}{Data-Efficient Learning}} & \multicolumn{4}{c}{Meta-Learning} \\
\cmidrule{2-5}          & \multicolumn{1}{c}{\multirow{3}[2]{*}{Adaptation}} & A Preference Learning Decoupling Framework for User Cold-Start Recommendation & SIGIR23 & UserCS* \\
          &       & CMML: Contextual Modulation Meta Learning for Cold-Start Recommendation & CIKM21 & UserCS* \\
          &       & MAMO: Memory-Augmented Meta-Optimization for Cold-start Recommendation & KDD20 & CS* \\
\cmidrule{2-5}          & \multicolumn{1}{c}{\multirow{4}[2]{*}{Pretraining}} & MeLU: Meta-Learned User Preference Estimator for Cold-Start Recommendation & KDD19 & CS* \\
          &       & Meta-Learning for User Cold-Start Recommendation & IJCNN19 & UserCS* \\
          &       & FORM: Follow the Online Regularized Meta-Leader for Cold-Start Recommendation & SIGIR21 & UserCS* \\
          &       & PNMTA: A Pretrained Network Modulation and Task Adaptation Approach for User Cold-Start Recommendation & WWW22 & UserCS* \\
\cmidrule{2-5}          & \multicolumn{4}{c}{Meta-Task} \\
\cmidrule{2-5}          & \multicolumn{1}{c}{\multirow{3}[2]{*}{Task-difference}} & Modeling Preference as Weighted Distribution over Functions for User Cold-start Recommendation & CIKM23 & UserCS* \\
          &       & Meta-Learning with Adaptive Weighted Loss for Imbalanced Cold-Start Recommendation & CIKM23 & UserCS* \\
          &       & Task-Difficulty-Aware Meta-Learning with Adaptive Update Strategies for User Cold-Start Recommendation & CIKM23 & UserCS* \\
\cmidrule{2-5}          & \multicolumn{1}{c}{\multirow{4}[2]{*}{Task-relevance }} & M2EU: Meta Learning for Cold-start Recommendation via Enhancing User Preference Estimation & SIGIR23 & CS* \\
          &       & Task Similarity Aware Meta Learning for Cold-Start Recommendation & CIKM22 & ItemCS* \\
          &       & Task-adaptive Neural Process for User Cold-Start Recommendation & WWW21 & UserCS* \\
          &       & Personalized Adaptive Meta Learning for Cold-start User Preference Prediction & AAAI21 & UserCS* \\
\cmidrule{2-5}          & \multicolumn{4}{c}{Meta-Embedding} \\
\cmidrule{2-5}          & \multicolumn{2}{l|}{Learning to Warm Up Cold Item Embeddings for Cold-start Recommendation with Meta Scaling and Shifting Networks} & SIGIR21 & ItemCS* \\
          & \multicolumn{2}{l|}{Warm Up Cold-start Advertisements: Improving CTR Predictions via Learning to Learn ID Embeddings} & SIGIR19 & ItemCS \\
\cmidrule{2-5}          & \multicolumn{4}{c}{Sequential Time Aware} \\
\cmidrule{2-5}          & \multicolumn{2}{l|}{Multimodal Meta-Learning for Cold-Start Sequential Recommendation} & CIKM22 & UserCS* \\
          & \multicolumn{2}{l|}{A Dynamic Meta-Learning Model for Time-Sensitive Cold-Start Recommendations} & AAAI22 & UserCS* \\
          & \multicolumn{2}{l|}{Cold-start Sequential Recommendation via Meta Learner} & AAAI21 & ItemCS* \\
          & \multicolumn{2}{l|}{Sequential Recommendation for Cold-start Users with Meta Transitional Learning} & SIGIR21 & UserCS* \\
    \bottomrule
    \end{tabular}%
    }
  \label{tab:overview_content}%
\end{table}%

\subsection{Graph Relations}

\subsection{Domain Information}

\subsection{World Knowledge from Large Language Models}
